# Supplementary material for: Magnetically Controllable Topological Quantum Phase Transitions in Antiferromagnetic Topological Insulator MnBi$_2$Te$_4$
Source: arXiv:1905.00642 source file (2019-05-23)
Supplement: Supplementary file 1 [file SM.pdf]

# SUPPLEMENTAL MATERIAL

## METHODS

First-principles calculations were performed by Vienna *ab initio* Simulation Package [1] in the framework of density functional theory (DFT), using the projector augmented wave method. The plane-wave basis with an energy cutoff of 350 eV was used. Perdew-Burke-Ernzerhof (PBE) type gradient generalized approximation (GGA) was applied in exchange-correlation functional [2]. The GGA+$U$ method was introduced to treat localized $3d$ orbitals of Mn atoms, using $U$=4 eV as previously tested [3]. The structural relaxation, including lattice constants and atomic positions, was performed using a force criteria of 0.01eV/Å. Spin-orbit coupling was included in self-consistent electronic calculations. The DFT-D3 method was applied to properly describe van der Waals interactions [4]. The Monkhorst-Pack **k**-point meshes of $9\times9\times3$, $9\times9\times5$, and $7\times7\times1$ were adopted for self-consistent calculations of antiferromagnetic (AFM) bulk, ferromagnetic (FM) bulk, and thin films, respectively. Band structures were mainly computed by GGA+$U$ method, except for FM bulk, which was studied by the modified Becke-Johnson methods [5] according to our previous tests [3]. Tight-binding Hamiltonians were constructed from maximally localized Wannier functions, based on which edge-state calculations were performed with WannierTools package [6].

## AFM $MnBi_2Te_4$ BULK

### Mirror Chern number and AFM mirror topological crystalline insulator (TCI)

The existence of $M_x$ and $P\mathcal{T}$ symmetries enables a new topological classification characterized by mirror Chern number $\mathcal{C}_M$ [8]. Since $M_x$ is commutate with $P\mathcal{T}$, mirror eigenvalues $\pm i$ can be used to label the two-fold degeneracy protected by $P\mathcal{T}$. Then, if one of the doubly degenerate states is labeled by $+i$, the other would be labeled by $-i$, and vice versa. Thus one can define two Chern numbers $\mathcal{C}_{+i}$ and $\mathcal{C}_{-i}$ for $+i$ and $-i$ subspaces, respectively, on the $M_x$ invariant plane in momentum space. The total Chern number $\mathcal{C} = \mathcal{C}_{+i} + \mathcal{C}_{-i}$ is required to be zero by $P\mathcal{T}$ symmetry, but $\mathcal{C}_M = (\mathcal{C}_{+i} - \mathcal{C}_{-i})/2$ can be nonzero. Specifically for bulk $MnBi_2Te_4$ with AFM-$x$ order, there exists a topological band inversion at $\Gamma$, which leads to nonzero $\mathcal{C}_{\pm i}$ and thus $|\mathcal{C}_M| = 1$. This refers to a new topological phase, called AFM mirror TCI, which has gapless (111) surface protected by $M_x$ symmetry and gapless side surfaces protected by $S$ symmetry.

### Surface states

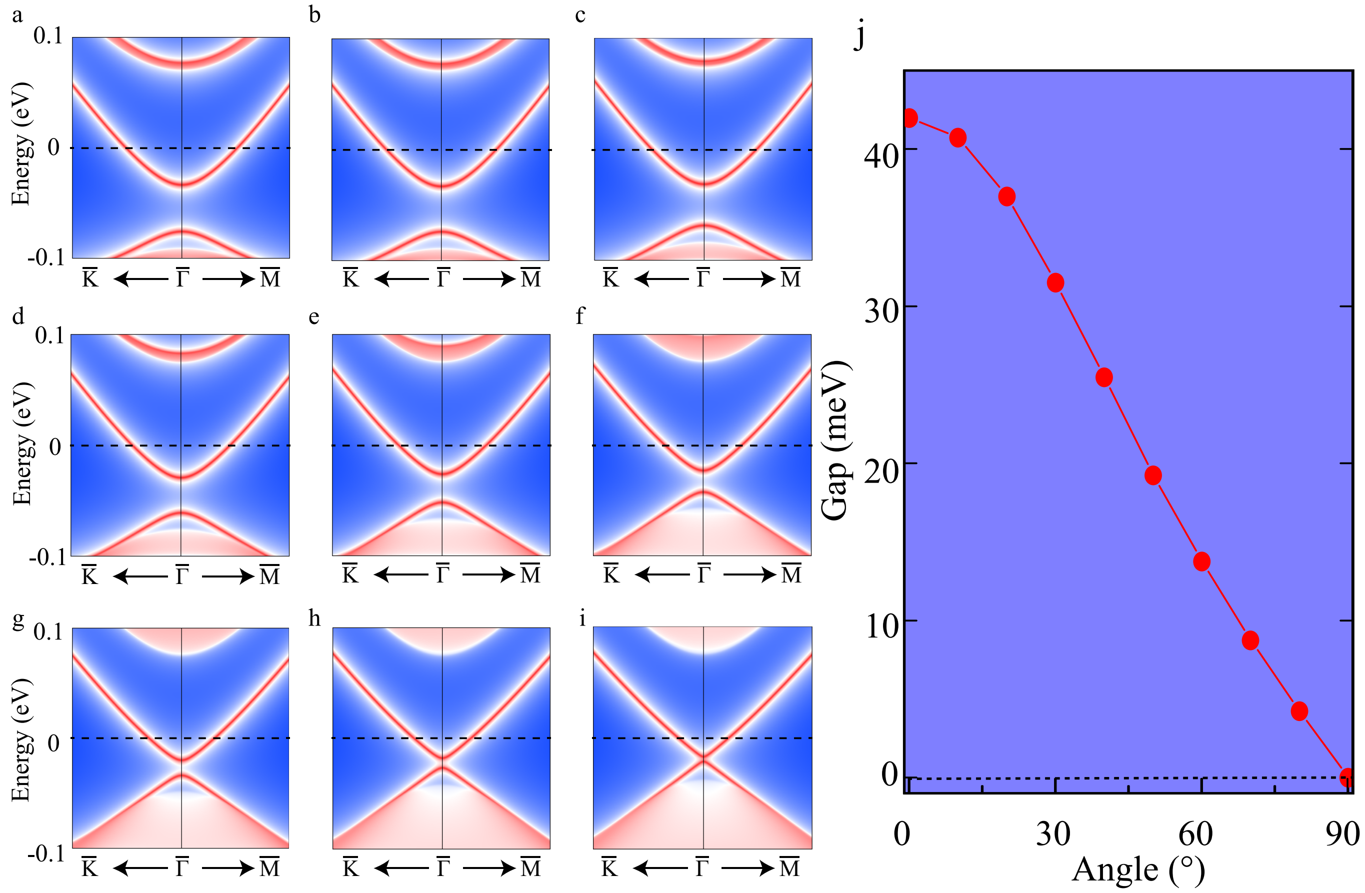


FIG. S1: (a-i) Surface states of AFM bulk $MnBi_2Te_4$ with different magnetic orientations, whose polar angles $\theta$ are 0°, 10°, 20°, 30°, 40°, 50°, 60°, 70° and 80°, respectively. (j) Surface-state band gaps of AFM $MnBi_2Te_4$ for different magnetic orientations.

## FM $MnBi_2Te_4$ BULK

TABLE S1: Evolution of Weyl points (WPs) in momentum space of FM $MnBi_2Te_4$ bulk when magnetic orientation rotates from out-of-plane to in-plane direction in the $k_x$-$k_z$ plane. Polar angle $\theta$ is defined in the spherical coordination, with 0°, 90°,and 180° representing $+z$, $+x$ and $-z$ directions, respectively.

| Angle (°) | $k_x$ (Å$^{-1}$) | $k_z$ (Å$^{-1}$) | Type |
|---|---|---|---|
| 0 | 0 | 0.0595 | Type-II |
| 10 | 0.0016 | 0.0585 | Type-II |
| 20 | 0.0032 | 0.0560 | Type-I |
| 30 | 0.0045 | 0.0518 | Type-I |
| 40 | 0.0056 | 0.0467 | Type-I |
| 50 | 0.0063 | 0.0404 | Type-I |
| 60 | 0.0064 | 0.0331 | Type-I |
| 70 | 0.0056 | 0.0245 | Type-I |
| 80 | 0.0037 | 0.0146 | Tpye-I |
| 90 | - | - | - |
| 100 | 0.0039 | -0.0151 | Type-I |
| 110 | 0.0058 | -0.0249 | Type-I |
| 120 | 0.0065 | -0.0332 | Type-I |
| 130 | 0.0065 | -0.0404 | Type-I |
| 140 | 0.0058 | -0.0469 | Type-I |
| 150 | 0.0048 | -0.0520 | Type-I |
| 160 | 0.0034 | -0.0562 | Type-I |
| 170 | 0.0018 | -0.0586 | Type-II |
| 180 | 0 | -0.0595 | Type-II |

TABLE S2: Evolution of Weyl points (WPs) in momentum space of FM $MnBi_2Te_4$ bulk when magnetic orientation rotates from out-of-plane to in-plane direction in the $k_y$-$k_z$ plane. Polar angle $\theta$ is defined in the spherical coordination, with 0°, 90°, and 180° representing $+z$, $+y$ and $-z$ directions, respectively.

| Angle (°) | $k_y$ (Å$^{-1}$) | $k_z$ (Å$^{-1}$) | Type |
|---|---|---|---|
| 0 | 0 | 0.0595 | Type-II |
| 10 | 0.0016 | 0.0586 | Type-II |
| 20 | 0.0031 | 0.0560 | Type-I |
| 30 | 0.0043 | 0.0520 | Type-I |
| 40 | 0.0052 | 0.0469 | Type-I |
| 50 | 0.0058 | 0.0402 | Type-I |
| 60 | 0.0058 | 0.0333 | Type-I |
| 70 | 0.0052 | 0.0251 | Type-I |
| 80 | 0.0034 | 0.0152 | Tpye-I |
| 90 | - | - | - |
| 100 | 0.0042 | -0.0145 | Type-I |
| 110 | 0.0064 | -0.0243 | Type-I |
| 130 | 0.0070 | -0.0404 | Type-I |
| 140 | 0.0062 | -0.0465 | Type-I |
| 150 | 0.0050 | -0.0520 | Type-I |
| 160 | 0.0035 | -0.0561 | Type-I |
| 170 | 0.0018 | -0.0586 | Type-II |
| 180 | 0 | -0.0595 | Type-II |

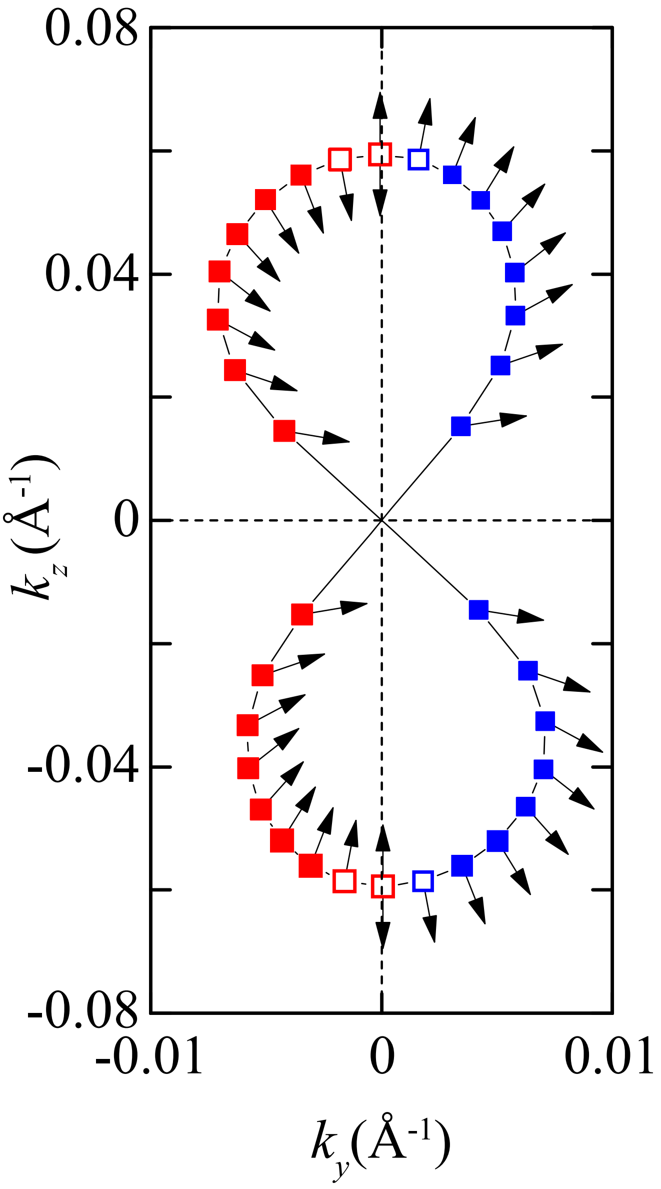


FIG. S2: Evolution of Weyl points (WPs) in momentum space of FM $MnBi_2Te_4$ bulk when magnetic orientation (denoted by black arrows) rotates from out-of-plane to in-plane direction in the $k_y$-$k_z$ plane. The closed and open squares denote type-I and type-II WPs, respectively. The blue and red colors represent topological charges of $+1$ and $-1$ carried by WPs.

## MNBI$_2$TE$_4$ FILMS

For the AFM-$x$ state, ultrathin films are an insulator with zero Chern number, while thick films are gapless as required by $M_x$ symmetry. For the later case, the breaking of $M_x$, for instance, by changing magnetic orientation or by applying strain, could open the band gap and might generate topological nontrivial phases [7]. For the AFM-$z$ state, previous work found that Chern number of $MnBi_2Te_4$ changes in an unique oscillating behavior between even and odd layers, giving rise to axion insulators and QAH insulators, respectively [3].

TABLE S3: Bandgap and Chern number ($\mathcal{C}$) of FM-$z$ $MnBi_2Te_4$ thin films with different thickness.

| | 3-SL | 4-SL | 5-SL | 6-SL | 7-SL | 8-SL |
|---|---|---|---|---|---|---|
| Gap (meV) | 78 | 76 | 63 | 57 | 49 | 46 |
| $\mathcal{C}$ | 1 | 1 | 1 | 1 | 1 | 1 |

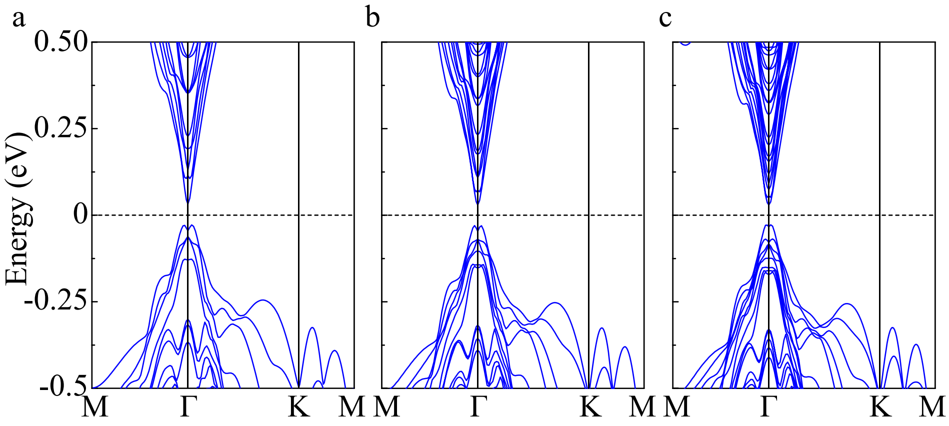


FIG. S3: Band structures of 3-SL, 4-SL and 5-SL FM-$z$ $MnBi_2Te_4$ thin films, respectively.

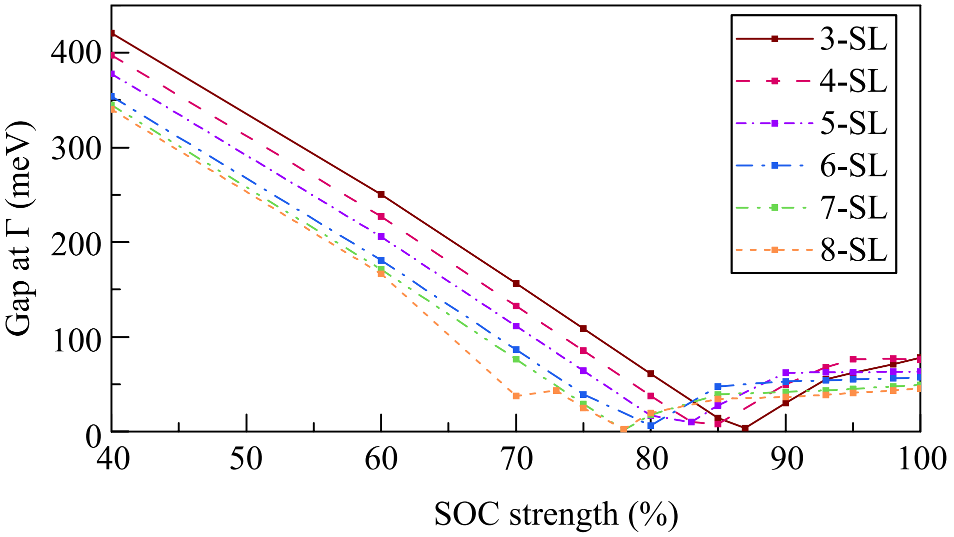


FIG. S4: Evolution of bandgap at Γ as a function of artificial spin-orbit coupling (SOC) strength for FM-$z$ $MnBi_2Te_4$ thin films from 3-SL to 8-SL.

[1] G. Kresse and J. Furthmüller, Phys. Rev. B **54**, 11169 (1996).
[2] J. P. Perdew, K. Burke, and M. Ernzerhof, Phys. Rev. Lett. **77**, 3865 (1996).
[3] J. Li, Y. Li, S. Du, Z. Wang, B.-L. Gu, S.-C. Zhang, K. He, W. Duan, and Y. Xu, arXiv:1808.08608 (2018).
[4] S. Grimme, J. Antony, S. Ehrlich, and H. Krieg, J. Chem. Phys. **132**, 154104 (2010).
[5] A. Becke and E. Johnson, J. Chem. Phys. **124**, 221101 (2006).
[6] Q. Wu, S. Zhang, H.-F. Song, M. Troyer, and A. A. Soluyanov, Comput. Phys. Commun. **224**, 405 (2018).
[7] X. Liu, H.-C. Hsu, and C.-X. Liu, Phys. Rev. Lett. **111**, 086802 (2013).
[8] J. C. Y. Teo, L. Fu, and C. L. Kane, Phys. Rev. B **78**, 045426 (2008).
